# Supplementary material for: A Survey on Robotic Prosthetics: Neuroprosthetics, Soft Actuators, and Control Strategies
Source: arXiv:2408.01729 source file (2024-08-03)
Supplement: Supplementary file 1 [file SupplimentaryMaterial.pdf]

# Appendix – Supplementary material for e-pub

## 2.1 Neuroprosthetics

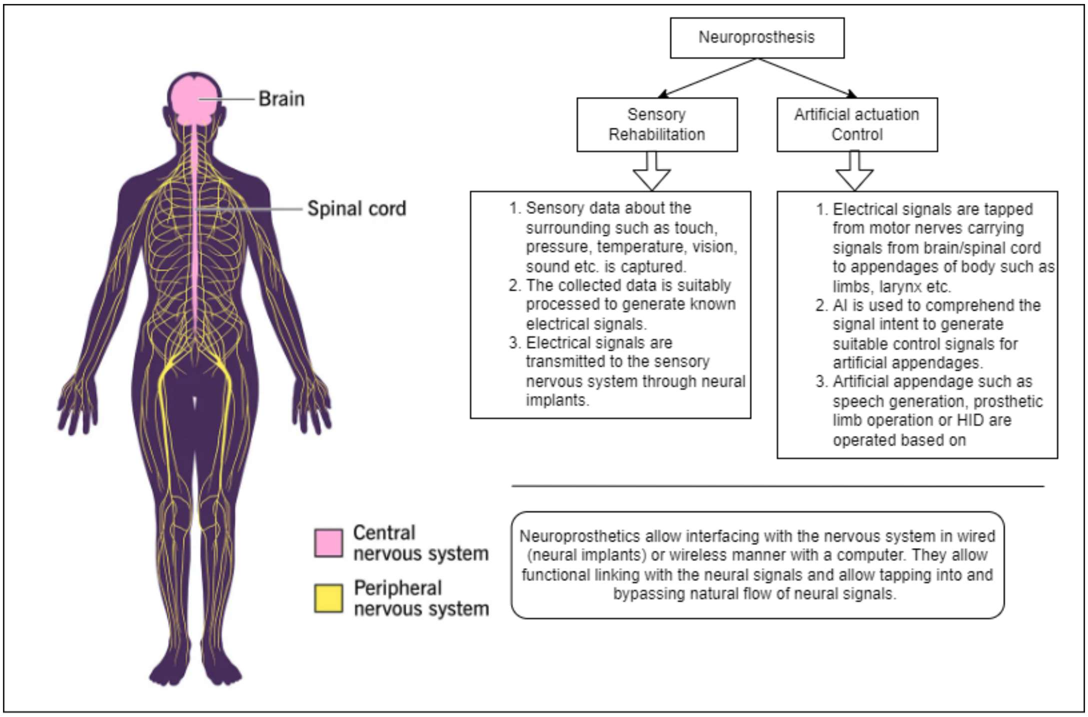


**Figure 1:** Overview of neural prosthesis applications.

---

### 2.1.1 Visual Prosthesis

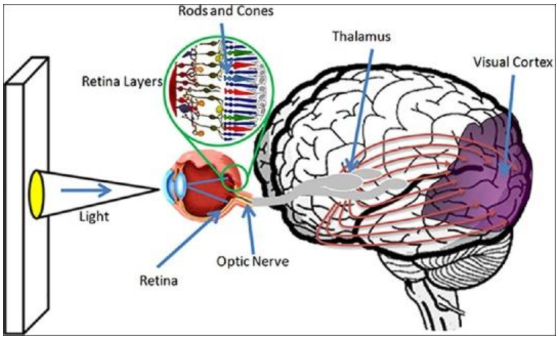


(a) Sites available for prosthetic application along visual pathway[7]

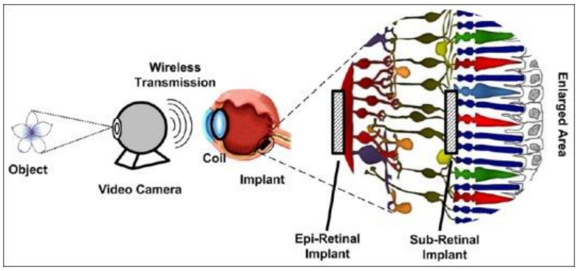


(b) Epiratinal Visual Prostheses [7]

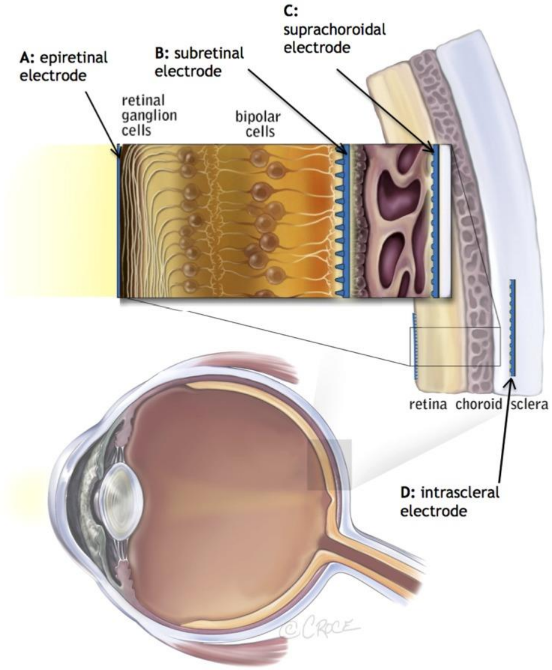


(c) Anatomy of human eye w.r.t. retinal prosthesis[4]

**Figure 2:** Visual Prostheses.

---

## 2.1.2 Visual Prosthesis

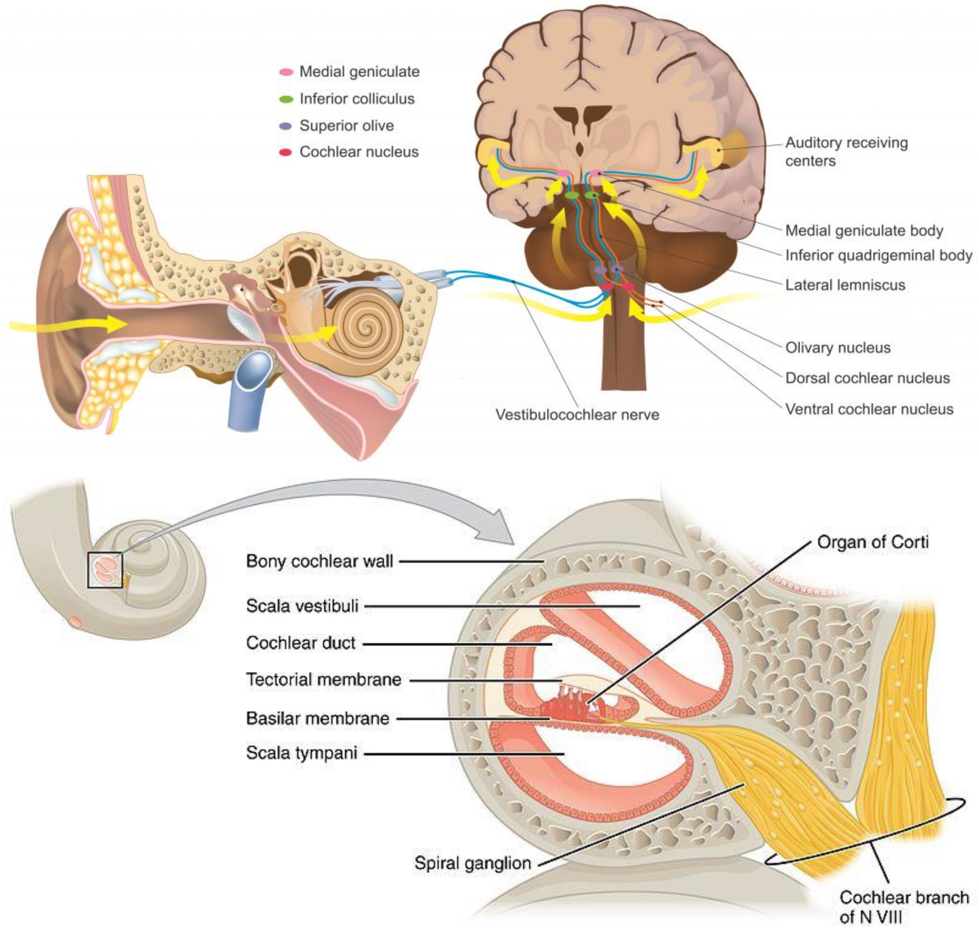


**Figure 3:** Auditory Pathway. [1]

---

## 3.2 Soft Robotics

| Parameter | Description | Value |
|---|---|---|
| Young's modulus | Austenite ($E_A$) | 75 GPa |
| | Martensite ($E_M$) | 28 GPa |
| Phase transformation temperature | Austenite start ($T_{As}$) | 68 °C |
| | Austenite finish $(T_{Af})$ | 78 °C |
| | Martensite start ($T_{Ms}$) | 52 °C |
| | Martensite finish ($T_{Mf}$) | 42 °C |
| Specific heat capacity | C | 0.322 J/g °C |
| Maximum deformation ratio | $\varepsilon_{max}$ | 8% |

**Figure 4:** Transition values of Nitinol SMA. [14]

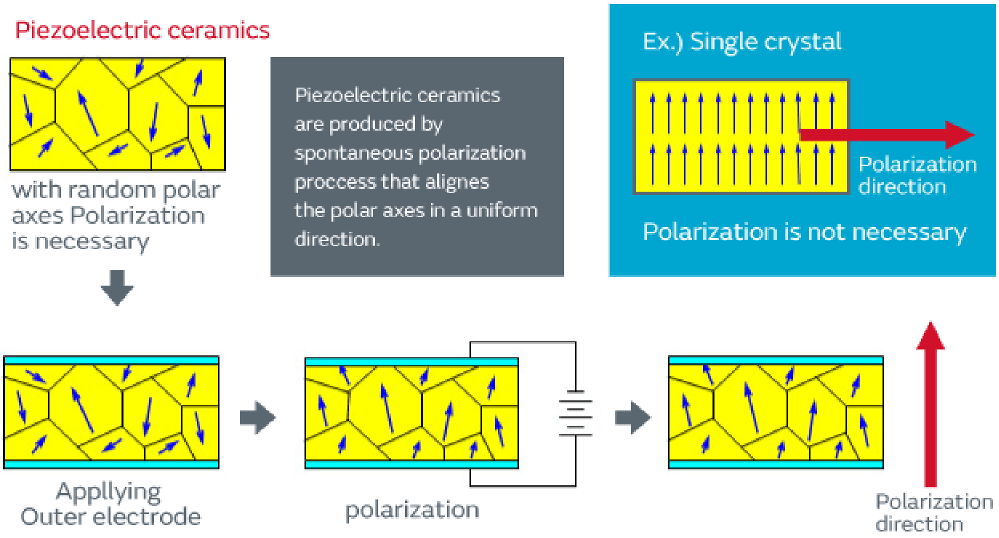


**Figure 8:** Principle of Piezoelectric Actuators. [6]

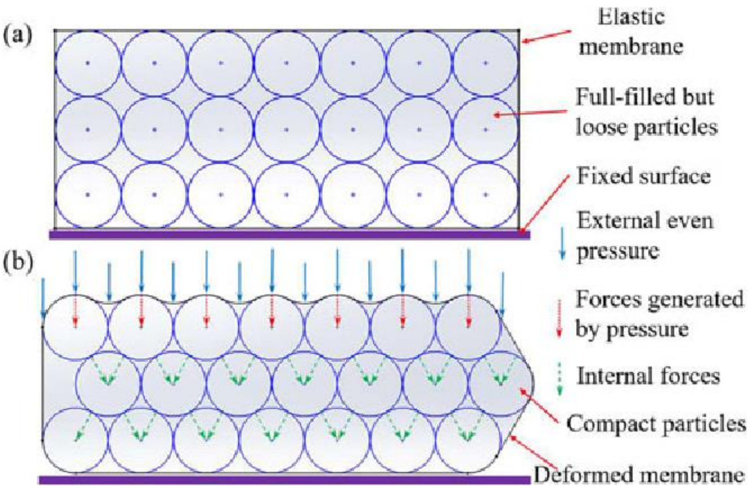


(a) Concept of Material Jamming Actuators(MJA). [11]

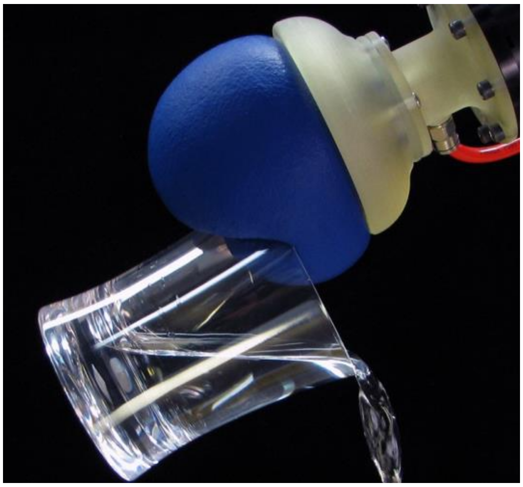

(b) Gripper based on MJA. [5]

**Figure 6:** Material Jamming Actuators. [8]

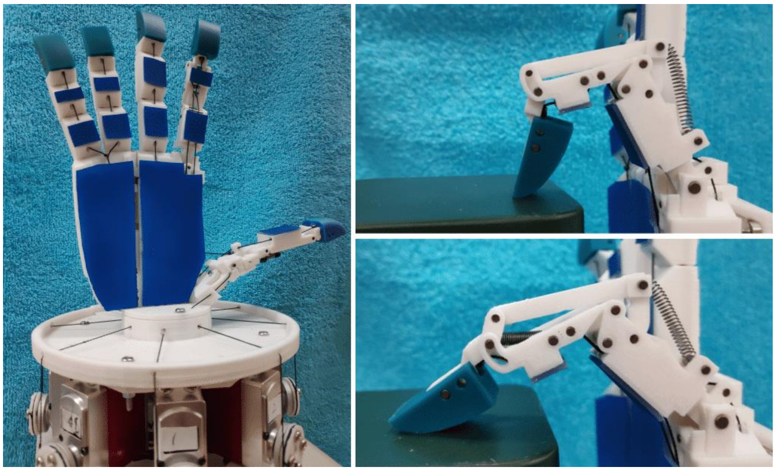

**Figure 7:** Design of a 9-actuator 19-DOF Anthropomorphic Robotic Hand. [15]

# 4 Control Strategies

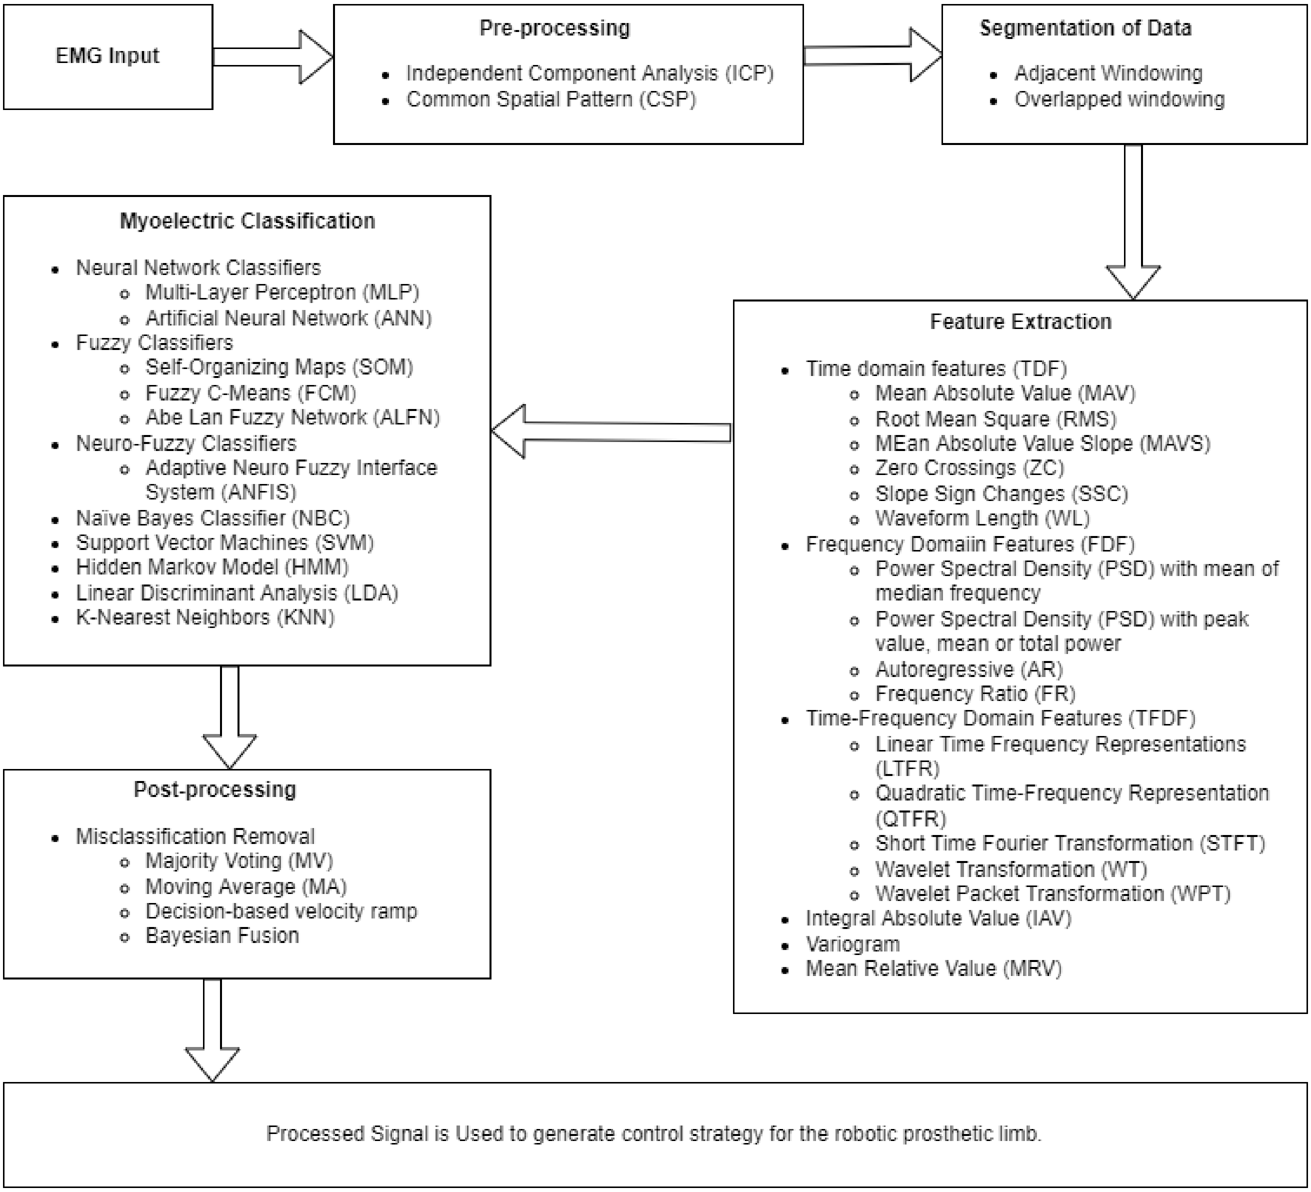


**Figure 8:** Computational Schema for preparation and processing of EMG signals for real-time prosthetic control. [12]

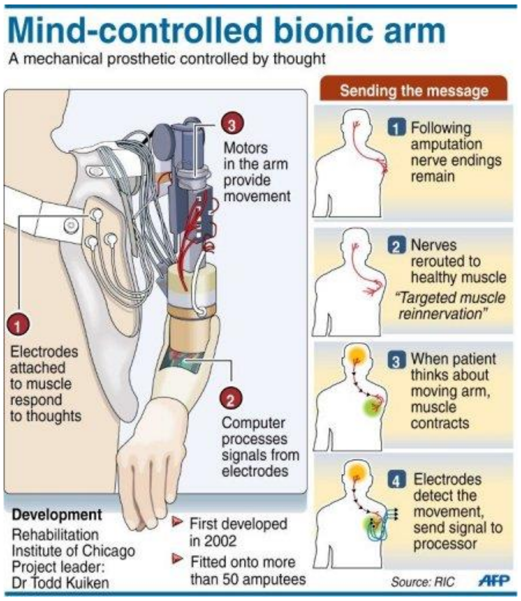


(a)

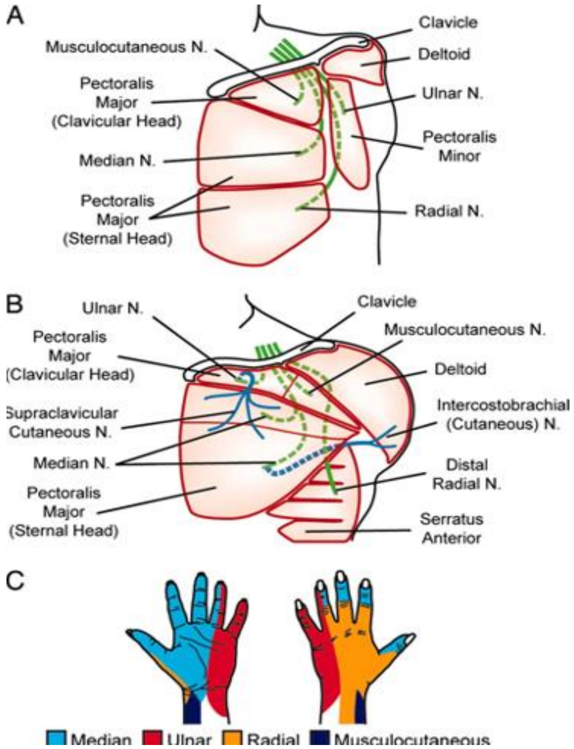


(b)

**Figure 9:** (a) A popular sketch of bionic arm control schema using TMR and EMG[2] (b) Concept Sketches of Targeted Muscle Reinnervation for arm amputation by Kuiken et al. 2004, 2007

---

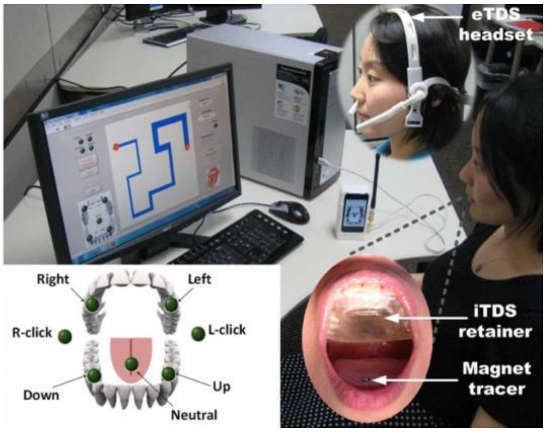


(a) eTDS Demonstration [9]

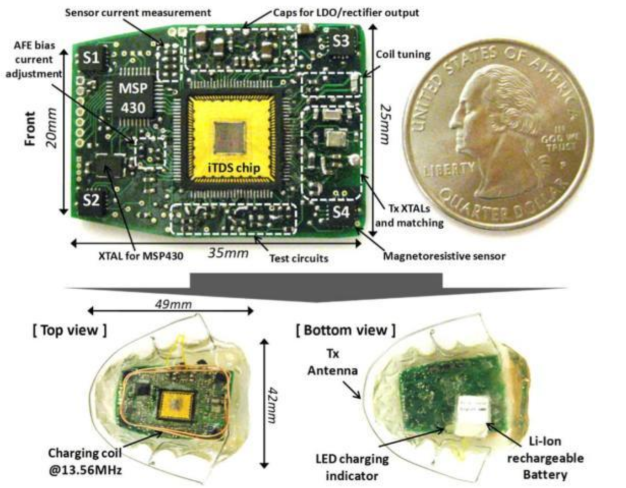


(c) iTDS based dental retainer [13]

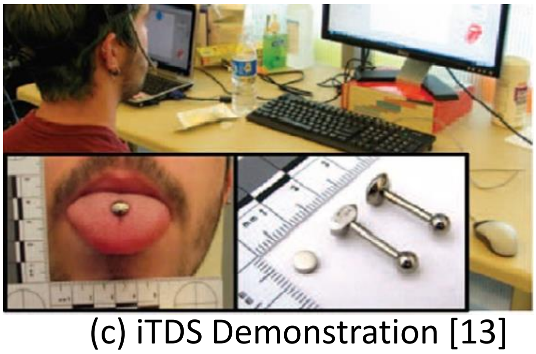

(c) iTDS Demonstration [13]

**Figure 10:** Tongue Driven System – HMI for prosthesis control

## 5 Parallel Trends

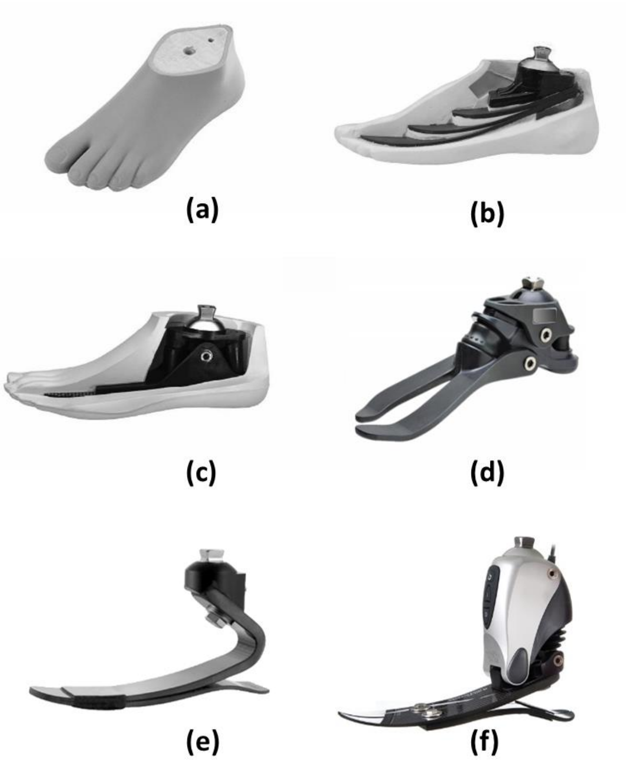


**Figure 11:** (a): SACH Foot, (b): Dynamic SACH Foot, (c): Single Axis Foot, (d): Multi-Axis Foot, (e): Passive-elastic Foot, (f): Powered Foot. Types of Prosthetic Foot-Ankle assemblies available commercially. [3]

---

# References


1. The auditory pathway. https://teachmeanatomy.info/neuroanatomy/pathways/auditory-pathway/. [Accessed: 2022-08-29 05:45:18]
2. Biomedinova: May 2012. http://biomedinova.blogspot.com/20120501archive.html [Accessed: 2022–08–29 04:42:01].
3. Feet and Ankles — pw.co.nz. https://www.pw.co.nz/products/categories/feet-and-ankles . [Accessed 14-Sep-2022].
4. Figure - pmc. https://www.ncbi.nlm.nih.gov/pmc/articles/PMC4270734/figure/pone-0115239-g001/ . [Accessed: 2022-08-29 05:49:21].
5. Jamming gripper - creative machines lab - columbia university https://www.creativemachineslab.com/jamming-gripper.html [Accessed: 2022-10-19 15:51:30].
6. Principles of piezoelectric actuators — actuator — murata manufacturing co., ltd. https://www.murata.com/en-global/products/mechatronics/actuator/overview/basic . [Accessed: 2022-08-28 02:51:00].
7. Visual prostheses: The enabling technology to give sight to the blind - pmc. https://www.ncbi.nlm.nih.gov/pmc/articles/PMC4329712/ . [Accessed: 2022-08-29 05:52:03].
8. Annabestani, M. and Fardmanesh, M. (2019). Ionic electro active polymer-based soft actuators and their applications in microfluidic micropumps, microvalves, and micromixers: A review.
9. Kim, J., Park, H., Bruce, J., Sutton, E., Rowles, D., Pucci, D., Holbrook, J., Minocha, J., Nardone, B., West, D., Laumann, A., Roth, E., Jones, M., Veledar, E., and Ghovanloo, M. (2013). The tongue enables computer and wheelchair control for people with spinal cord injury. Science Translational Medicine, 5(213).

10. Kuiken, T. A., Miller, L. A., Lipschutz, R. D., Lock, B. A., Stubblefield, K., Marasco, P. D., Zhou, P., and Dumanian, G. A. (2007). Targeted reinnervation for enhanced prosthetic arm function in a woman with a proximal amputation: a case study. The Lancet, 369(9559):371–380.
11. Li, Y., Chen, Y., Yang, Y., and Wei, Y. (2017). Passive particle jamming and its stiffening of soft robotic grippers. IEEE Transactions on Robotics, 33(2):446–455.
12. Parajuli, N., Sreenivasan, N., Bifulco, P., Cesarelli, M., Savino, S., Niola, V., Esposito, D., Hamilton,T. J., Naik, G. R., Gunawardana, U., and Gargiulo, G. D. (2019). Real-time EMG based pattern recognition control for hand prostheses: A review on existing methods, challenges and future implementation. Sensors, 19(20):4596
13. Park, H., Kiani, M., Lee, H.-M., Kim, J., Block, J., Gosselin, B., and Ghovanloo, M. (2012). A wireless magnetoresistive sensing system for an intraoral tongue-computer interface. IEEE Transactions on Biomedical Circuits and Systems, 6(6):571–585.
14. Park, H.-B., Kim, D.-R., Kim, H.-J., Wang, W., Han, M.-W., and Ahn, S.-H. (2019). Design and analysis of artificial muscle robotic elbow joint using shape memory alloy actuator. International Journal of Precision Engineering and Manufacturing, 21(2):249–256.
15. Zhang, Z., Han, T., Pan, J., and Wang, Z. (2018). Catch-919 hand: Design of a 9-actuator 19-dof anthropomorphic robotic hand.
